# Supplementary material for: Region-Constrained Group Relative Policy Optimization for Flow-Based Image Editing
Source: arXiv:2604.09386 source file (2026-09-03)
Supplement: Supplementary file 1 [file supp.tex]

%%%%%%%% ECCV 2026 SUPPLEMENTARY FILE %%%%%%%%%%%%%%%%%

\documentclass[runningheads]{llncs}

% ---------------------------------------------------------------
% Include basic ECCV package
\usepackage[review,year=2026,ID=10116]{eccv}

% ---------------------------------------------------------------
% Other packages
\usepackage{eccvabbrv}
\usepackage{microtype}
\usepackage{graphicx}
\usepackage{booktabs}
\usepackage{tabularx}
\usepackage{array}
\usepackage{placeins}
\usepackage{amsmath}
\usepackage{amssymb}
\usepackage{amsfonts}
\usepackage{algorithm}
\usepackage{algorithmic}
\usepackage{capt-of}
\usepackage[pagebackref,breaklinks,colorlinks,citecolor=eccvblue]{hyperref}

\newcolumntype{Y}{>{\raggedleft\arraybackslash}X}
\newcolumntype{L}{>{\raggedright\arraybackslash}X}

\begin{document}

\title{Region-Constrained Group Relative Policy Optimization for Flow-Based Image Editing}
\titlerunning{Supplementary Material}
\author{Anonymous Authors}
\authorrunning{Anonymous Authors}
\institute{Anonymous Institution}
\maketitle

\appendix
\numberwithin{equation}{section}
\renewcommand{\theequation}{\thesection.\arabic{equation}}
\renewcommand{\theHequation}{\thesection.\arabic{equation}}

% =========================================================
\section{Variance Reduction Analysis for Region-Decoupled Perturbation}
\label{app:proof_prop1}
% =========================================================

This appendix provides a local justification for Proposition~\ref{prop:variance_reduction}
via linearization and the delta method.
We focus on the \emph{conditional} intra-group reward variance given the shared reference noise $\epsilon^\ast$,
which directly governs the sample standard deviation used in group-standardized advantages.
For self-containment, we restate the GRPO group-standardized advantage used in the main paper:
\begin{equation}
A_i=\frac{r_i-\mathrm{mean}(\{r_1,\ldots,r_G\})}{\mathrm{std}(\{r_1,\ldots,r_G\})}.
\label{eq:grpo_adv_supp}
\end{equation}
All approximation errors and higher-order cross-region couplings are collected into
$\Delta_{\mathrm{interaction}}$.

\begin{proposition}[Global perturbation induces nuisance variance; RDP suppresses it]
\label{prop:variance_reduction}
Fix a deterministic solver, yielding a deterministic map $x_0=\Phi_\theta(\epsilon,c)$.
Let $\epsilon^\ast$ be a shared reference initial noise and consider candidates $\{\epsilon^{(i)}\}_{i=1}^G$
constructed around $\epsilon^\ast$.

Under local smoothness and weak cross-region sensitivity (Eq.~\eqref{eq:struct_assump_app}),
the background-only reward component $R_{\mathrm{base}}$ (Eq.~\eqref{eq:reward_bridge_app})
has first-order conditional variance scaling
\begin{equation}
\begin{aligned}
\mathrm{Var}[R_{\mathrm{base}}\mid \epsilon^\ast]
&\approx \sigma^2\|h\|_2^2,
&& \text{(global perturbation)},\\
\mathrm{Var}[R_{\mathrm{base}}\mid \epsilon^\ast]
&\approx \alpha_{\mathrm{base}}^2\|h\|_2^2,
&& \text{(RDP)}.
\end{aligned}
\end{equation}
where $h$ is the local gradient of $R_{\mathrm{base}}$ w.r.t.\ background noise
(Eq.~\eqref{eq:h_def_app}).
Hence, for $\alpha_{\mathrm{base}}<\sigma$ and $\|h\|_2>0$, RDP reduces background-induced nuisance variance
by a first-order factor $\approx \alpha_{\mathrm{base}}^2/\sigma^2$, improving the SNR of group-standardized
advantages in Eq.~\eqref{eq:grpo_adv_supp} and facilitating credit assignment for localized edits.
\end{proposition}

% ---------------------------------------------------------
\subsection{Deterministic Map and a Reward Bridge}
\label{app:struct_bridge}

\subsubsection*{Deterministic map.}
Under a fixed deterministic solver, sampling induces a deterministic map
\begin{equation}
x_0=\Phi_\theta(\epsilon,c),\qquad \epsilon\sim\mathcal N(0,I),
\end{equation}
where $\epsilon$ corresponds to the initial noise (i.e., $x_1$ in the ODE formulation).

\subsubsection*{Mask decomposition.}
Let $M\in\{0,1\}^D$ be the editing mask. For any $\epsilon$, define
\begin{equation}
\epsilon^{\mathrm{in}}=M\odot \epsilon,
\qquad
\epsilon^{\mathrm{base}}=(1-M)\odot \epsilon,
\label{eq:mask_decompose_app}
\end{equation}
We denote the anchor noise as $\epsilon^\ast$ and its decomposition as
$\epsilon^{\mathrm{in}\,*}$ and $\epsilon^{\mathrm{base}\,*}$.
For convenience, define the background-restricted identity
\begin{equation}
I_{\mathrm{base}} \triangleq \mathrm{Diag}(1-M).
\label{eq:ibase_def_app}
\end{equation}
We also write $x_0^{\mathrm{base}} \triangleq (1-M)\odot x_0$ when needed.

\subsubsection*{Weak cross-region sensitivity (structural assumption).}
Locally around $\epsilon^\ast$, we assume the background part of the terminal latent is weakly sensitive
to perturbations in the editing subspace:
\begin{equation}
\left\|
\frac{\partial x_0^{\mathrm{base}}}{\partial \epsilon^{\mathrm{in}}}
\right\|_F
\le
\kappa
\left\|
\frac{\partial x_0^{\mathrm{base}}}{\partial \epsilon^{\mathrm{base}}}
\right\|_F,
\qquad \kappa\ll 1.
\label{eq:struct_assump_app}
\end{equation}
Intuitively, within a small neighborhood, cross-region influence (edit $\rightarrow$ base)
is much weaker than within-region propagation (base $\rightarrow$ base).

\subsubsection*{Reward bridge.}
The main text defines an additive reward
\begin{equation}
R(x_0,c) = R_{\mathrm{edit}}(x_0,c) + R_{\mathrm{pres}}(x_0,c),
\end{equation}
where $R_{\mathrm{pres}}$ measures changes only in the background region.
Under Eq.~\eqref{eq:struct_assump_app} and local smoothness of $R_{\mathrm{pres}}$,
we adopt the following local insensitivity approximation:
\begin{equation}
\begin{aligned}
R_{\mathrm{pres}}(\Phi_\theta(\epsilon^{\mathrm{in}}+\epsilon^{\mathrm{base}},c),c)
&\approx
R_{\mathrm{pres}}(\Phi_\theta(\epsilon^{\mathrm{in}\,*}+\epsilon^{\mathrm{base}},c),c)\\
&\triangleq
R_{\mathrm{base}}(\epsilon^{\mathrm{base}};\epsilon^{\mathrm{in}\,*}).
\end{aligned}
\label{eq:reward_bridge_app}
\end{equation}
For brevity, we write $R_{\mathrm{base}}(\epsilon^{\mathrm{base}})$ when unambiguous.

\subsubsection*{Reward decomposition in $\epsilon$-space.}
Define the terminal reward as a function of $\epsilon$:
\begin{equation}
\tilde R(\epsilon)\triangleq R(\Phi_\theta(\epsilon,c),c).
\end{equation}
Using Eq.~\eqref{eq:reward_bridge_app}, we obtain the local decomposition
\begin{equation}
\begin{aligned}
\tilde R(\epsilon)
&\approx
\underbrace{R_{\mathrm{edit}}(\Phi_\theta(\epsilon,c),c)}_{\triangleq~\tilde R_{\mathrm{edit}}(\epsilon)}
+ R_{\mathrm{base}}(\epsilon^{\mathrm{base}})\\
&\quad + \Delta_{\mathrm{interaction}},
\end{aligned}
\label{eq:reward_decomp_app}
\end{equation}
where $\Delta_{\mathrm{interaction}}$ collects approximation errors and residual cross-region couplings
(e.g., attention leakage across regions).

% ---------------------------------------------------------
\subsection{Delta Method for Conditional Reward Variance}
\label{app:delta_method}

We analyze the intra-group conditional variance given the anchor $\epsilon^\ast$.
Let
\begin{equation}
\Delta\epsilon^{(i)} \triangleq \epsilon^{(i)}-\epsilon^\ast,
\qquad
x_0^\ast \triangleq \Phi_\theta(\epsilon^\ast,c).
\end{equation}
Linearizing the deterministic map around $\epsilon^\ast$ gives
\begin{equation}
\Phi_\theta(\epsilon^\ast+\Delta\epsilon,c)
\approx
x_0^\ast + J\,\Delta\epsilon,
\qquad
J \triangleq \frac{\partial \Phi_\theta(\epsilon,c)}{\partial \epsilon}\Big|_{\epsilon=\epsilon^\ast}.
\label{eq:lin_map_app}
\end{equation}
Applying the delta method to $\tilde R(\epsilon)$ at $\epsilon^\ast$ yields
\begin{equation}
\mathrm{Var}[\tilde R(\epsilon)\mid \epsilon^\ast]
\approx
a^\top \,\mathrm{Cov}[\Delta\epsilon\mid \epsilon^\ast]\, a,
\qquad
a \triangleq \nabla_{\epsilon}\tilde R(\epsilon)\Big|_{\epsilon=\epsilon^\ast}.
\label{eq:reward_var_delta_app}
\end{equation}
By the chain rule,
\begin{equation}
a = J^\top g_0,
\qquad
g_0 \triangleq \nabla_{x_0} R(x_0,c)\Big|_{x_0=x_0^\ast}.
\label{eq:chain_rule_app}
\end{equation}
Hence, differences between perturbation schemes are captured by
$\mathrm{Cov}[\Delta\epsilon\mid \epsilon^\ast]$, in particular the variance allocated to the
background subspace.

\subsubsection*{Variance decomposition under the reward bridge.}
Plugging Eq.~\eqref{eq:reward_decomp_app} into Eq.~\eqref{eq:reward_var_delta_app},
the conditional variance under \emph{global} perturbation can be written (up to $\Delta_{\mathrm{interaction}}$) as
\begin{equation}
\begin{aligned}
\mathrm{Var}_{\mathrm{global}}[\tilde R\mid \epsilon^\ast]
&\approx
\mathrm{Var}[\tilde R_{\mathrm{edit}}\mid \epsilon^\ast]
+
\underbrace{\mathrm{Var}[R_{\mathrm{base}}(\epsilon^{\mathrm{base}})\mid \epsilon^\ast]}_{\text{nuisance variance}}\\
&\quad+
2\,\mathrm{Cov}\!\Big(\tilde R_{\mathrm{edit}},\,R_{\mathrm{base}}\Big)
+
\Delta_{\mathrm{interaction}}.
\end{aligned}
\label{eq:var_global_app}
\end{equation}
Moreover, by Cauchy--Schwarz,
\begin{equation}
\Big|\mathrm{Cov}(\tilde R_{\mathrm{edit}},R_{\mathrm{base}})\Big|
\le
\sqrt{\mathrm{Var}(\tilde R_{\mathrm{edit}})\,\mathrm{Var}(R_{\mathrm{base}})}.
\label{eq:cov_bound_app}
\end{equation}
Thus, inflating $\mathrm{Var}(R_{\mathrm{base}})$ increases not only nuisance variance itself but also
a conservative upper bound on the edit--base covariance magnitude.

% ---------------------------------------------------------
\subsection{Global Perturbation Baseline}
\label{app:global}
We consider a global perturbation baseline similar in spirit to Neighbor GRPO~\cite{he2025neighbor}.

Neighbor GRPO uses global perturbation of the form
\begin{equation}
\epsilon^{(i)}=\sqrt{1-\sigma^2}\,\epsilon^\ast+\sigma\,\delta^{(i)},
\qquad \delta^{(i)}\sim\mathcal N(0,I).
\label{eq:global_noise_app}
\end{equation}
Conditioned on $\epsilon^\ast$, we have
\begin{equation}
\Delta\epsilon^{(i)}=\epsilon^{(i)}-\epsilon^\ast
=
\left(\sqrt{1-\sigma^2}-1\right)\epsilon^\ast+\sigma\delta^{(i)} ,
\end{equation}
and thus the conditional covariance is
\begin{equation}
\mathrm{Cov}[\Delta\epsilon\mid \epsilon^\ast]=\sigma^2 I.
\label{eq:cov_global_app}
\end{equation}
In particular, the background subspace receives the same variance scale $\sigma^2$,
which directly contributes to the nuisance variance term in Eq.~\eqref{eq:var_global_app}.

% ---------------------------------------------------------
\subsection{Region-Decoupled Perturbation Suppresses Nuisance Variance}
\label{app:local}

Our region-decoupled perturbation uses a shared reference noise $\epsilon^\ast$ and includes one unperturbed reference candidate.
Let $i_0\in\{1,\dots,G\}$ denote the reference index. We construct
\begin{equation}
\begin{aligned}
\epsilon^{(i_0)} &= \epsilon^\ast,\\
\epsilon^{(i)} &= \sqrt{1-\boldsymbol{\alpha}^2}\odot \epsilon^\ast
+\boldsymbol{\alpha}\odot \delta^{(i)},\qquad i\neq i_0,\\
\boldsymbol{\alpha} &= \alpha_{\mathrm{edit}}M+\alpha_{\mathrm{base}}(1-M),
\end{aligned}
\label{eq:local_noise_app}
\end{equation}
where $\delta^{(i)}\sim\mathcal N(0,I)$ are i.i.d.\ for $i\neq i_0$.

Conditioned on $\epsilon^\ast$, for $i\neq i_0$ we have
\begin{equation}
\Delta\epsilon^{(i)}=\epsilon^{(i)}-\epsilon^\ast
=
\left(\sqrt{1-\boldsymbol{\alpha}^2}-\mathbf{1}\right)\odot \epsilon^\ast
+
\boldsymbol{\alpha}\odot \delta^{(i)},
\end{equation}
where $\mathbf{1}$ is the all-ones vector (and operations are element-wise).
Therefore, for $i\neq i_0$ the conditional covariance is
\begin{equation}
\mathrm{Cov}[\Delta\epsilon^{(i)}\mid \epsilon^\ast]=\mathrm{Diag}(\boldsymbol{\alpha}^2).
\label{eq:cov_local_app}
\end{equation}
The reference candidate $i_0$ has $\Delta\epsilon^{(i_0)}=\mathbf{0}$ and thus does not introduce additional conditional variance.
Notably, the background-subspace variance scale is reduced from $\sigma^2$ (global perturbation) to $\alpha_{\mathrm{base}}^2$ (RDP).

\subsubsection*{Nuisance variance scaling.}
Under the reward bridge (Eq.~\eqref{eq:reward_bridge_app}), $R_{\mathrm{base}}$ varies only with
$\epsilon^{\mathrm{base}}$ when $\epsilon^{\mathrm{in}\,*}$ is fixed.
Linearizing $R_{\mathrm{base}}$ around $\epsilon^{\mathrm{base}\,*}$ yields
\begin{equation}
\begin{aligned}
R_{\mathrm{base}}(\epsilon^{\mathrm{base}\,*}+\Delta\epsilon^{\mathrm{base}})
&\approx
R_{\mathrm{base}}(\epsilon^{\mathrm{base}\,*}) + h^\top \Delta\epsilon^{\mathrm{base}},\\
h
&\triangleq
\nabla_{\epsilon^{\mathrm{base}}}R_{\mathrm{base}}(\epsilon^{\mathrm{base}})
\Big|_{\epsilon^{\mathrm{base}}=\epsilon^{\mathrm{base}\,*}}.
\end{aligned}
\label{eq:h_def_app}
\end{equation}
Under region-decoupled perturbation, $\Delta\epsilon^{\mathrm{base}}\sim\mathcal N(0,\alpha_{\mathrm{base}}^2 I_{\mathrm{base}})$, so
\begin{equation}
\mathrm{Var}_{\mathrm{local}}[R_{\mathrm{base}}\mid \epsilon^\ast]
\approx
h^\top (\alpha_{\mathrm{base}}^2 I_{\mathrm{base}})\,h
=
\alpha_{\mathrm{base}}^2 \|h\|_2^2.
\label{eq:var_base_local_app}
\end{equation}
Under global perturbation, $\Delta\epsilon^{\mathrm{base}}\sim\mathcal N(0,\sigma^2 I_{\mathrm{base}})$, so
\begin{equation}
\mathrm{Var}_{\mathrm{global}}[R_{\mathrm{base}}\mid \epsilon^\ast]
\approx
h^\top (\sigma^2 I_{\mathrm{base}})\,h
=
\sigma^2 \|h\|_2^2.
\label{eq:var_base_global_app}
\end{equation}
Therefore,
\begin{equation}
\begin{aligned}
\mathrm{Var}_{\mathrm{local}}[R_{\mathrm{base}}\mid \epsilon^\ast]
&<
\mathrm{Var}_{\mathrm{global}}[R_{\mathrm{base}}\mid \epsilon^\ast],\\
\text{with first-order reduction factor }
&\approx \alpha_{\mathrm{base}}^2/\sigma^2.
\end{aligned}
\label{eq:var_base_reduce_app}
\end{equation}
This proves the stated local scaling and explains why suppressing background perturbations improves the SNR of
group-standardized advantages in Eq.~\eqref{eq:grpo_adv_supp}.

% ---------------------------------------------------------
\subsection{Connection to Process-Level Constraints (ACD)}
\label{app:acd_link}

$\Delta_{\mathrm{interaction}}$ also captures residual cross-region couplings accumulated along ODE integration
(e.g., attention leakage), which may still affect background preservation even when $\alpha_{\mathrm{base}}\approx 0$.
This motivates the process-level intrinsic reward ACD introduced in the main paper to further suppress such interactions,
extending ``localized exploration at initialization'' to ``dynamic localization throughout the entire trajectory''.

% =========================================================
\section{Technical Appendix (Scheme B): Region-Normalized Masked Metric (Candidate-Set Surrogate Policy)}
\label{app:schemeB_masked_cov}
% =========================================================

\noindent
This appendix rewrites the derivation of the surrogate policy on the candidate set under \textbf{Scheme B}:
we define a surrogate leaping policy used only during training on the candidate set with the region-normalized
masked metric $d_C^2$, which is equivalent to a masked Gaussian kernel with a fixed covariance normalized by mask size.
We focus on (i) the leaping kernel and its posterior responsibilities under this metric; and
(ii) the engineering form used to compute $\log\pi_\theta$ and policy ratios in GRPO.

% ---------------------------------------------------------
\subsection{Notation}
\label{app:schemeB_notation}

Let the latent at time $t\in[0,1]$ be $x_t\in\mathbb{R}^D$.
Let $M\in\{0,1\}^D$ denote a flattened editing mask ($1$ = editable, $0$ = background), and define
\begin{equation}
D_M \triangleq \mathrm{diag}(M),\qquad I-D_M=\mathrm{diag}(1-M).
\end{equation}
\begin{equation}
\bar M \triangleq 1-M,\qquad |M| \triangleq \sum_{d=1}^D M_d,\qquad |\bar M| \triangleq \sum_{d=1}^D \bar M_d.
\end{equation}

We use a region-normalized (masked) Mahalanobis distance with optional bandwidth parameters
$\tau_{\mathrm{edit}},\tau_{\mathrm{base}}>0$:
\begin{equation}
\begin{split}
d_C^2(x,y;M;\tau_{\mathrm{edit}},\tau_{\mathrm{base}})
&=
\frac{\|M\odot(x-y)\|_2^2}{(|M|+\varepsilon)\,\tau_{\mathrm{edit}}^2}\\
&\quad+
\frac{\|\bar M\odot(x-y)\|_2^2}{(|\bar M|+\varepsilon)\,\tau_{\mathrm{base}}^2},
\end{split}
\label{eq:dc_metric_app}
\end{equation}
where $\varepsilon=10^{-8}$ is used for numerical stability.
Here $\tau_{\mathrm{edit}}$ and $\tau_{\mathrm{base}}$ are region-wise bandwidth parameters
that control the relative sensitivity of the surrogate policy to deviations inside and outside
the editing region, respectively. Smaller values make the corresponding region contribute more
sharply to the surrogate responsibilities.

\subsubsection*{Discrete-time note (numerical stability).}
All derivations below are applied at discrete solver timesteps $\{t_k\}_{k=1}^{T}$ with $t_k\in(0,1]$.
When expressions contain factors like $1/t$, we implicitly operate on $t_k\ge t_{\min}>0$
(e.g., by excluding $t=0$ from the update schedule or clamping), which avoids numerical explosion at the final step.

% ---------------------------------------------------------
\subsection{Masked Leaping Kernel and Responsibilities}
\label{app:schemeB_leaping}

We use a Gaussian kernel only as a convenient way to express the quadratic score; the surrogate policy
is instantiated as a softmax over candidate distances.

\subsubsection*{Leaping kernel.}
Define a masked Gaussian kernel
\begin{equation}
\pi(x_t\mid x_t')=\mathcal{N}(x_t\mid x_t',\Sigma_C),
\qquad
\Sigma_C=(|M|+\varepsilon)\tau_{\mathrm{edit}}^{2}D_M+(|\bar M|+\varepsilon)\tau_{\mathrm{base}}^{2}(I-D_M).
\end{equation}
Equivalently,
\begin{equation}
\Sigma_C^{-1}=
\frac{1}{(|M|+\varepsilon)\tau_{\mathrm{edit}}^{2}}D_M
+\frac{1}{(|\bar M|+\varepsilon)\tau_{\mathrm{base}}^{2}}(I-D_M).
\end{equation}

\subsubsection*{Monte-Carlo mixture and posterior responsibilities.}
Given $G$ candidates $x_t^{(i)}=\Phi_{1\to t}(\epsilon^{(i)};\theta_{\mathrm{old}},c)$,
the mixture approximation is
\begin{equation}
\hat\pi(x_t)=\frac{1}{G}\sum_{i=1}^G \pi(x_t\mid x_t^{(i)}).
\end{equation}
Assuming a uniform prior over candidates, Bayes' rule yields responsibilities
\begin{equation}
\begin{aligned}
\hat\pi(x_t^{(i)}\mid x_t)
&=
\frac{\pi(x_t\mid x_t^{(i)})}{\sum_{j=1}^G \pi(x_t\mid x_t^{(j)})}\\
&=
\mathrm{softmax}_i\!\left(
-\frac{1}{2}(x_t-x_t^{(i)})^\top\Sigma_C^{-1}(x_t-x_t^{(i)})
\right)\\
&=
\mathrm{softmax}_i\!\left(
-\frac{1}{2}d_C^2(x_t,x_t^{(i)};M;\tau_{\mathrm{edit}},\tau_{\mathrm{base}})
\right).
\end{aligned}
\label{eq:schemeB_responsibilities}
\end{equation}

\subsubsection*{Effect of region normalization.}
With diagonal $\Sigma_C$, the exponent expands as
\begin{equation}
(x_t-x_t^{(i)})^\top\Sigma_C^{-1}(x_t-x_t^{(i)})
=
\frac{\|D_M(x_t-x_t^{(i)})\|_2^2}{(|M|+\varepsilon)\tau_{\mathrm{edit}}^{2}}
+
\frac{\|(I-D_M)(x_t-x_t^{(i)})\|_2^2}{(|\bar M|+\varepsilon)\tau_{\mathrm{base}}^{2}},
\end{equation}
so each region contributes its mean squared error, removing the linear dependence of the logits on region size
and reducing mask-dependent temperature drift.

% ---------------------------------------------------------
\subsection{Engineering Form: Surrogate Policy over $G$ Candidates}
\label{app:schemeB_engineering}

In practical GRPO, we instantiate the surrogate leaping policy over the $G$ candidates within a group.
Conditioning on an anchor index $k$ sampled uniformly from the perturbed candidate set $\mathcal I=\{1,\dots,G\}\setminus\{i_0\}$ and using the center under the current parameters
$x_t^{(\theta,k)}=\Phi_{1\to t}(\epsilon^{(k)};\theta,c)$, we define
\begin{equation}
\pi_\theta\!\left(x_t^{(i)} \mid s_t,k\right)
=
\frac{
\exp\!\left(
-\frac{1}{2}\,d_C^2\!\left(x_t^{(i)},x_t^{(\theta,k)};M;\tau_{\mathrm{edit}},\tau_{\mathrm{base}}\right)
\right)
}{
\sum_{j=1}^G
\exp\!\left(
-\frac{1}{2}\,d_C^2\!\left(x_t^{(j)},x_t^{(\theta,k)};M;\tau_{\mathrm{edit}},\tau_{\mathrm{base}}\right)
\right)
}.
\label{eq:schemeB_policy_app}
\end{equation}
Here $s_t=\{x_t^{(1)},\dots,x_t^{(G)}\}$ is the candidate set rolled out under $\theta_{\mathrm{old}}$.
Any global scalar factor (e.g., the $1/2$) may be absorbed into the distance scale,
as long as the same convention is used consistently for $\log\pi_\theta$ and policy ratios in the GRPO objective.

\paragraph{Bandwidth calibration.}
The bandwidth parameters $(\tau_{\mathrm{edit}},\tau_{\mathrm{base}})$ control the softness of the surrogate
responsibilities and, in turn, the sharpness of the policy ratios.
In ablations, we consider a perturbation-calibrated setting,
$\tau_{\mathrm{edit}}=c\,\alpha_{\mathrm{edit}}$ and $\tau_{\mathrm{base}}=\max(c\,\alpha_{\mathrm{base}},\tau_{\min})$
(with $\tau_{\min}=10^{-3}$ for numerical stability), which aligns the kernel bandwidth with the typical candidate deviations
induced by anisotropic initial-noise perturbations.
In our main experiments, we use $\tau_{\mathrm{edit}}=0.9$ and $\tau_{\mathrm{base}}=1.1$, while other combinations are evaluated in the main paper's ablation studies.

\section{Experimental Settings and Hyperparameters}
\label{app:exp_details}

\begin{table}[h]
    \centering
    \caption{Experimental settings and hyperparameters for GRPO post-training.}
    \vspace{2pt}
    \label{tab:hyperparams}
    \begin{tabularx}{\columnwidth}{@{}lc@{}}
        \toprule
        \textbf{Hyperparameter / Setting} & \textbf{Value} \\
        \midrule
        Group size $G$ & $8$ \\
        Anchors per group $B$ & $2$ \\
        Sampling steps (train) $T_{\mathrm{train}}$ & $12$ \\
        Sampling steps (eval) $T_{\mathrm{eval}}$ & $28$ \\
        RDP coefficients & $\alpha_{\mathrm{edit}}=0.3$, $\alpha_{\mathrm{base}}=10^{-4}$ \\
        Surrogate bandwidths $(\tau_{\mathrm{edit}},\tau_{\mathrm{base}})$ & $(0.9,\;1.1)$ \\
        Global perturbation strength $\sigma$ (baseline only) & $0.3$ \\
        ACD layer set $\mathcal{L}_{\mathrm{sel}}$ & $\{10,11,\dots,19\}$ \\
        Learning rate & $3\times 10^{-4}$ \\
        Batching (prompts per update) & $64$ \\
        LoRA rank & $64$ \\
        Reward weights $(\lambda_{\mathrm{task}},\lambda_{\mathrm{acd}})$ & $(0.5,\;0.5)$ \\
        \bottomrule
    \end{tabularx}
    \vspace{-6pt}
\end{table}

The GRPO objective in the main paper is written in its general clipped-ratio form with an optional KL regularization term. In our implementation, we set the KL coefficient to $\beta=0$.

For each rollout $i$, we compute a task reward $R_{\mathrm{task}}^{(i)}$ using EditScore~\cite{luo2025editscore} and an intrinsic reward $R_{\mathrm{acd}}^{(i)}$ from Eq.~\eqref{eq:acd_reward_supp}. Since the two reward terms have different scales, we normalize them separately across the minibatch:
\begin{equation}
\hat R_{\mathrm{task}}^{(i)}
=
\frac{R_{\mathrm{task}}^{(i)}-\mu_{\mathrm{task}}}{\sigma_{\mathrm{task}}+\varepsilon},
\qquad
\hat R_{\mathrm{acd}}^{(i)}
=
\frac{R_{\mathrm{acd}}^{(i)}-\mu_{\mathrm{acd}}}{\sigma_{\mathrm{acd}}+\varepsilon},
\end{equation}
where $(\mu_{\mathrm{task}},\sigma_{\mathrm{task}})$ and $(\mu_{\mathrm{acd}},\sigma_{\mathrm{acd}})$ denote the minibatch mean and standard deviation of the corresponding reward term. The final rollout reward is then computed as
\begin{equation}
R^{(i)}
=
\lambda_{\mathrm{task}} \hat R_{\mathrm{task}}^{(i)}
+
\lambda_{\mathrm{acd}} \hat R_{\mathrm{acd}}^{(i)}.
\label{eq:final_reward_supp}
\end{equation}
Group-standardized advantages are finally computed from the set of final rewards $\{R^{(i)}\}_{i=1}^{G}$ using Eq.~\eqref{eq:grpo_adv_supp}.

\section{Additional Diagnostics}
\label{app:diagnostics}

For self-containment, we restate the ACD definition used in the main paper.
Let $A^{(i)}_{l,t}(v,u)$ denote the text-to-image cross-attention weight at layer $l$ and step $t$.
We define the attention mass received by image token $u$ as
\begin{equation}
a^{(i)}_{l,t}(u)=\sum_v A^{(i)}_{l,t}(v,u).
\label{eq:acd_mass_supp}
\end{equation}
The relative attention density inside the editing mask is
\begin{equation}
\mathrm{ACD}^{(i)}_{l,t}
=
\frac{
\frac{1}{|M|+\varepsilon}\sum_u a^{(i)}_{l,t}(u)\,M(u)
}{
\frac{1}{N_{\mathrm{img}}+\varepsilon}\sum_u a^{(i)}_{l,t}(u)
}.
\label{eq:acd_def_supp}
\end{equation}
The intrinsic reward is defined by aggregating ACD over selected layers and sampling steps:
\begin{equation}
R_{\mathrm{acd}}^{(i)}
=
\frac{1}{|\mathcal{L}_{\mathrm{sel}}|\,T}
\sum_{l\in\mathcal{L}_{\mathrm{sel}}}\sum_{t=1}^{T}\mathrm{ACD}^{(i)}_{l,t}.
\label{eq:acd_reward_supp}
\end{equation}

\subsection{Layer-wise ACD Residual on FLUX.1-Kontext-dev}
\label{app:acd_diag}

\begin{figure}[t]
\centering
\includegraphics[width=\linewidth, trim=20mm 30mm 20mm 30mm, clip]{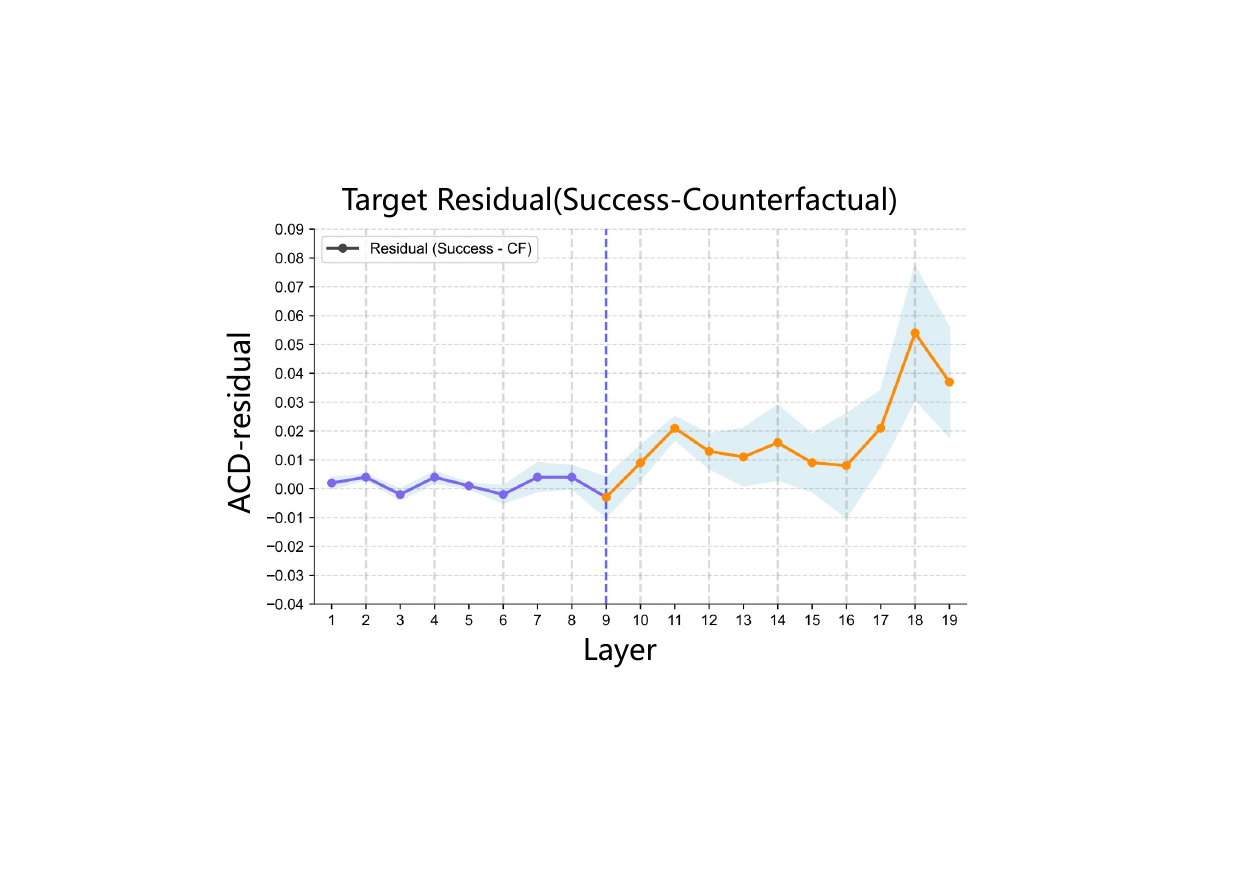}
\caption{\textbf{Layer-wise ACD residual on FLUX.1-Kontext-dev.}
We plot $\Delta_l$ in Eq.~\eqref{eq:acd_residual_def}, the mean ACD difference between successful and failed rollouts.
Separation becomes stronger in late layers, supporting the predefined set of late layers $\mathcal{L}_{\mathrm{sel}}$.}
\label{fig:acd_residual}
\end{figure}

This appendix provides a diagnostic analysis that motivates the predefined layer set
$\mathcal{L}_{\mathrm{sel}}$ used in the ACD intrinsic reward (Eq.~\eqref{eq:acd_reward_supp}).
The analysis is \emph{not} used for tuning: we fix $\mathcal{L}_{\mathrm{sel}}$ as the last $K$ cross-attention
layers in all experiments and report this diagnostic only to justify that late layers carry a cleaner region-grounding signal.
For FLUX.1-Kontext-dev~\cite{labs2025flux}, we consider the dual-stream transformer blocks for this diagnostic; the model uses 19 dual-stream blocks, so the predefined set $\mathcal{L}_{\mathrm{sel}}=\{10,\dots,19\}$ corresponds to the last 10 dual-stream blocks.

\subsubsection*{Setup.}
For a subset of prompts, we sample multiple deterministic ODE rollouts by perturbing the initial noise, and obtain a scalar task score for each rollout using the official EditScore implementation, consistent with training. Specifically, we use 200 prompts and generate 4 rollouts per prompt. For each prompt, we select the highest-scoring rollout as \emph{positive} and the lowest-scoring rollout as \emph{negative}.

\subsubsection*{Per-layer residual.}
For each rollout $i$, layer $l$, and step $t$, we compute $\mathrm{ACD}^{(i)}_{l,t}$ by Eq.~\eqref{eq:acd_def_supp},
and aggregate over steps:
\begin{equation}
\overline{\mathrm{ACD}}^{(i)}_{l} \triangleq \frac{1}{T}\sum_{t=1}^{T}\mathrm{ACD}^{(i)}_{l,t}.
\end{equation}
Let $\mathcal{P}$ and $\mathcal{N}$ denote the positive and negative rollout sets, respectively.
We define the \emph{layer-wise ACD residual} as the mean difference
\begin{equation}
\Delta_l \triangleq
\mathbb{E}_{i\sim \mathcal{P}}\!\left[\overline{\mathrm{ACD}}^{(i)}_{l}\right]
-
\mathbb{E}_{i\sim \mathcal{N}}\!\left[\overline{\mathrm{ACD}}^{(i)}_{l}\right].
\label{eq:acd_residual_def}
\end{equation}
A larger $\Delta_l$ indicates that successful rollouts exhibit stronger attention concentration in the editing region at layer $l$.

\subsubsection*{Observation.}
Fig.~\ref{fig:acd_residual} shows that $\Delta_l$ is small in early layers and becomes consistently larger in late layers,
suggesting that late cross-attention layers provide a more separable region-grounding signal.
This supports our design choice to compute $R_{\mathrm{acd}}$ over a fixed set of late layers.

\clearpage
\section{More Qualitative Comparisons}
\label{app:more_qual}
\vspace{13pt}

\begin{center}
    \includegraphics[width=\linewidth,height=0.95\textheight,keepaspectratio]{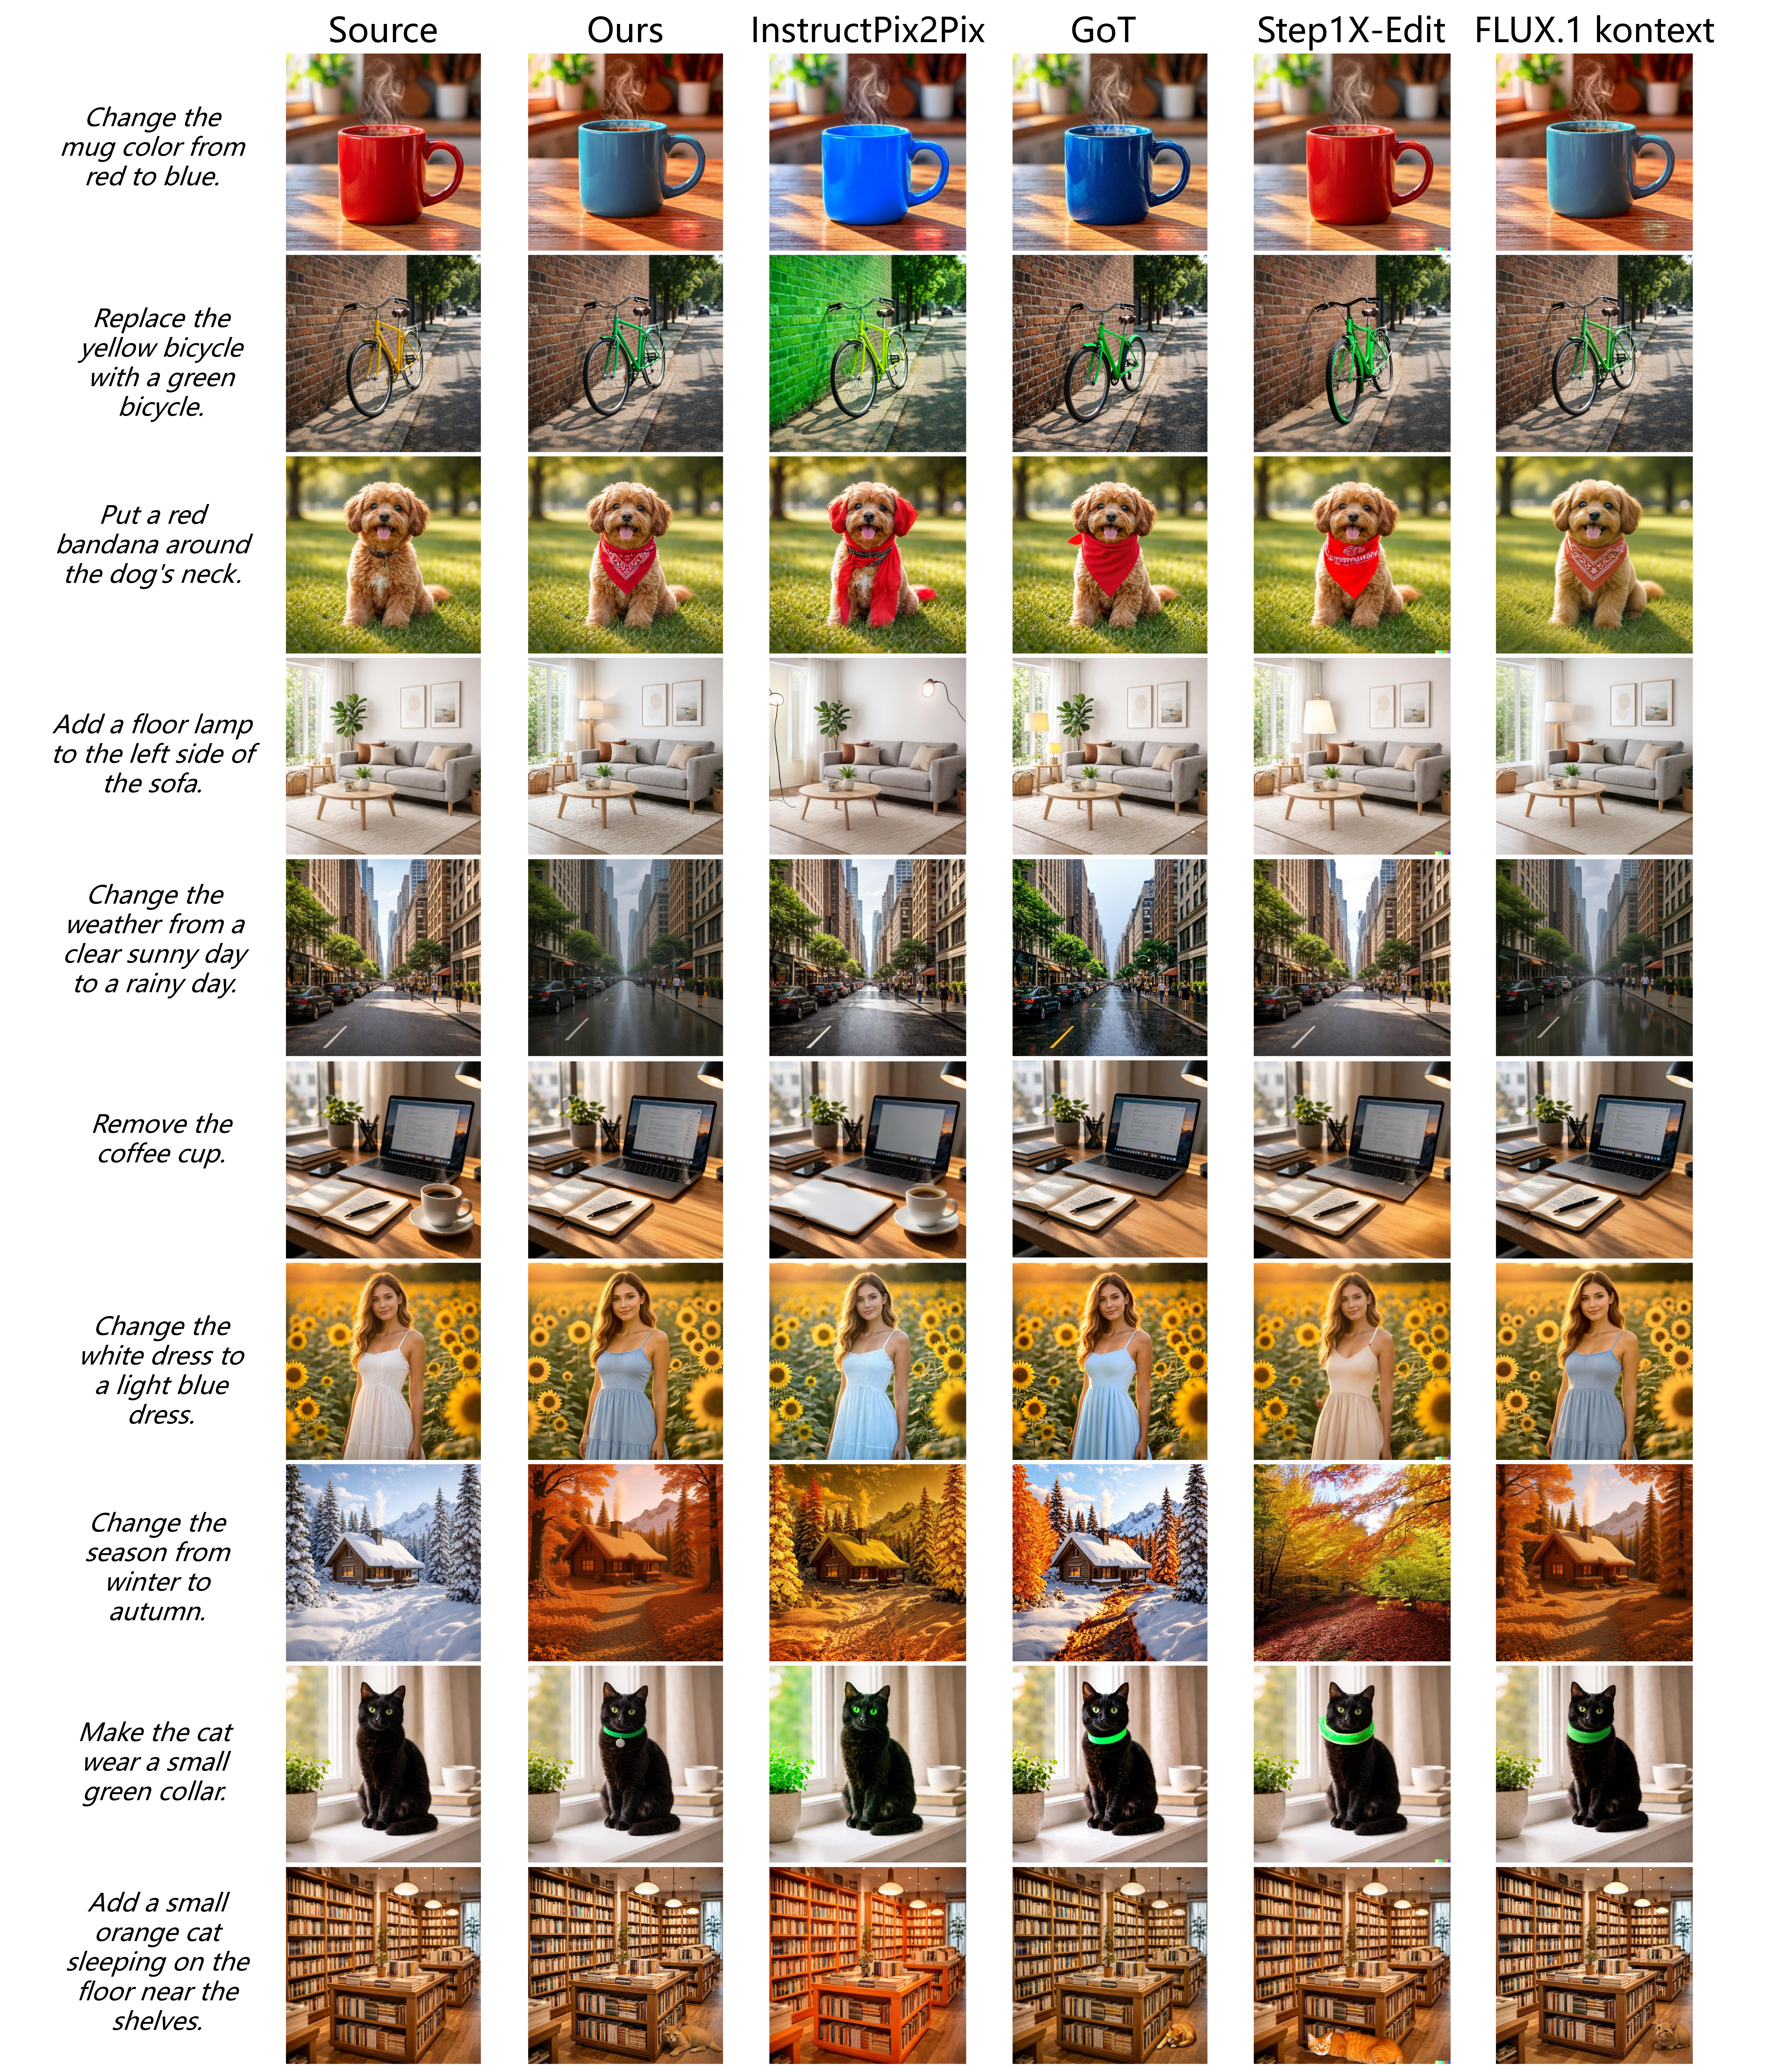}
    \captionof{figure}{\textbf{More qualitative comparisons on CompBench~\cite{jia2025compbench}.}
    Additional examples across Add/Remove/Replace tasks.
    Each row shows the source image, the editing instruction, and outputs from different editors.
    Our method yields stronger edit-region faithfulness while better preserving non-target content.}
    \label{fig:more_qualitative}
\end{center}

\clearpage

\bibliographystyle{splncs04}
\bibliography{main}

\end{document}
